# Supplementary material for: A Memory-Efficient Sketch Method for Estimating High Similarities in Streaming Sets
Source: arXiv:1905.08977 source file (2019-05-22)
Supplement: Supplementary file 1 [file appendix.tex]

\section*{Appendix}\label{sec:appendix}
\subsection*{Pseudo-code of Our Algorithm}
\begin{algorithm}[h]
	\SetKwRepeat{Do}{do}{while}%
	\SetKwFunction{EstimateJaccard}{EstimateJaccard}
	\SetKwFunction{UpdateUIPair}{UpdateUIPair}
	\SetKwFunction{continue}{continue}
	\SetKwInOut{Input}{input}
	\SetKwInOut{Output}{output}
	\Input{$\Pi, k, \alpha = 0.7213$.}
	\BlankLine
	
	$U\gets \emptyset$\;
	\ForEach{user-item pair $(u,v)$ arriving on stream $\Pi$}{
		\UpdateUIPair($u, v$)\;
	}
	\BlankLine
	\textbf{Function} \UpdateUIPair($u, v$)\\
	\If {$u\notin U$} {
		$U\gets U \cup \{u\}$\;
		\For {$i \in \{1,\ldots,k\}$}{
			$s_u[i]\gets 1$\;
			$m_u[i] \gets \lfloor -  \log_2 h_i (v) \rfloor$\;
		}
	}
	\Else{
		\For {$i \in \{1,\ldots,k\}$}{
			$r_i(v) \gets \lfloor -  \log_2 h_i (v) \rfloor$\;
			\If {$r_i(v) \ge m_u[i]$} {
				\If {$r_i(v) == m_u[i]$} {
					$s_u[i]\gets 0$\;
					\continue()\;
				}
				$s_u[i] \gets 1$\;
				$m_u[i] \gets r_i(v)$\;
			}
		}
	}
	\BlankLine
	%\tcc{\EstimateJaccard($u_1, u_2$) returns the Jaccard simialrity of users $u_1$ and $u_2$ at the current time.}
	\textbf{Function} \EstimateJaccard($u_1, u_2$)\\
	$\hat k\gets 0$\;
	\For {$i \in \{1,\ldots,k\}$}{
		\If {$m_{u_1}[i] == m_{u_2} [i]$} {
			\continue()\;
		}
		\If {$m_{u_1}[i] > m_{u_2} [i]$ and $s_{u_1}[i] == 1$} {
			$\hat k \gets \hat k + 1$\;
			\continue()\;
		}
		\If {$m_{u_1}[i] < m_{u_2}[i]$ and $s_{u_2}[i] == 1$} {
			$\hat k \gets \hat k + 1$\;
		}
	}
	$\hat J_{u_1, u_2} \gets 1 - \hat k k^{-1}\alpha^{-1}$\;
	\caption{The pseudo-code of MaxLogHash. \label{alg:MaxLogHash}}
\end{algorithm}
\subsection*{Proof of Theorem~\ref{theorem: prob}}
	Let $r^*$ be the maximum log-rank of all items in $\cup (u_1, u_2)$.
	When two items $w$ and $v$ in $I_{u_1}$ or $I_{u_2}$ has the log-rank value $r^*$,
	we easily find that $\psi_{u_1, u_2} [i]=0$.
	When only one item $w$ in $I_{u_1}$ and only one item $v$ in $I_{u_2}$ have the log-rank value $r^*$,
	we easily find that $\chi_{u_1, u_2} [i]=0$.
	Let
	\[
	\Delta(u_1, u_2) = (I_{u_1}\setminus I_{u_2}) \cup (I_{u_2}\setminus I_{u_1}) =\cup (u_1, u_2) \setminus \cap(u_1, u_2).
	\]
	Then, we find that event $\chi_{u_1, u_2} [i] = 1 \wedge \psi_{u_1, u_2} [i] = 1$ happens (i.e., $\delta_{u_1, u_2} [i]=1$) only when one item $w$ in $\Delta(u_1, u_2)$ has a log-rank value larger than all items in $\cup (u_1, u_2)\setminus \{w\}$.
	For any item $v\in I$, we have $h_i(v)\sim Uniform(0, 1)$ and so $r_i(v)\sim Geometric(1/2)$,
	supported on the set $\{0, 1, 2, \ldots\}$.
	Based on the above observations, when $|\cup(u_1, u_2)|\ge 2$, we have
	\begin{equation*}
	\begin{split}
	&P(\delta_{u_1, u_2} [i]=1 \wedge r^* = j) \\
	&= \sum_{w\in \Delta(u_1, u_2)} P(r_i(w) = j) \prod_{v\in \cup (u_1, u_2)\setminus \{w\}}  P(r_i(v) < j)\\
	&= \frac{|\Delta(u_1, u_2)|}{2^{j+1}}\left(1-\frac{1}{2^j}\right)^{|\cup(u_1, u_2)|-1}.
	\end{split}
	\end{equation*}
	Therefore, we have
	\begin{equation*}
	\begin{split}
	&P(\delta_{u_1, u_2} [i]=1)=\sum_{j=0}^{+\infty} P(\delta_i = 1\wedge r^* = j) \\
	&= \sum_{w\in \Delta(u_1, u_2)} P(r_w = j) \prod_{v\in \cup (u_1, u_2)\setminus \{w\}}  P(r_v < j)\\
	&= \sum_{j=0}^{+\infty} \frac{|\Delta(u_1, u_2)|}{2^{j+1}}\left(1-\frac{1}{2^j}\right)^{|\cup(u_1, u_2)|-1}\\
	&= \sum_{j=1}^{+\infty} \frac{|\Delta(u_1, u_2)|}{|\cup(u_1, u_2)|} \cdot \frac{|\cup(u_1, u_2)|}{2^{j+1}}\left(1-\frac{1}{2^j}\right)^{|\cup(u_1, u_2)|-1}\\
	&=\alpha_{|\cup(u_1, u_2)|} (1-J_{u_1, u_2}),
	\end{split}
	\end{equation*}
	where the last equation holds because $|\Delta(u_1, u_2)| = |\cup(u_1, u_2)| - |\cap(u_1, u_2)|$.
\subsection*{Proof of Theorem~\ref{theorem: error}}
	From equation~(\ref{eq:expk}), we  easily have
	\begin{equation*}
	\begin{split}
	\mathbb{E}(\hat J_{u_1, u_2}) &=\mathbb{E}\left(1 - \frac{\hat k}{k\alpha}\right)\\
	&=1 - \frac{k \alpha_{|\cup(u_1, u_2)|} (1-J_{u_1, u_2})}{k \alpha}\\
	&=\beta_{|\cup(u_1, u_2)|} J_{u_1, u_2} + 1 - \beta_{|\cup(u_1, u_2)|}.
	\end{split}
	\end{equation*}
	To derive $\text{Var}(\hat J_{u_1, u_2})$, we first compute
	\begin{eqnarray*}
		\mathbb{E}(\hat k^2) &=& \mathbb{E}\left(\left(\sum_{i=1}^k \mathbf{1} (\delta_{u_1, u_2} [i]=1)\right)^2\right) \\
		&=&\sum_{i=1}^k \mathbb{E}\left((\mathbf{1} (\delta_{u_1, u_2} [i]=1))^2 \right) \\
		&&+\sum_{i\ne j, 1\le i,j\le k} \mathbb{E}\left(\mathbf{1} (\delta_{u_1, u_2} [i]=1) \mathbf{1} (\delta_{u_1, u_2} [j]=1) \right) \\
		&=& k \alpha_{|\cup(u_1, u_2)|} (1-J_{u_1, u_2}) + k (k-1) \alpha_{|\cup(u_1, u_2)|}^2 (1-J_{u_1, u_2})^2.
	\end{eqnarray*}
	Then, we have
	\begin{eqnarray}\label{eq:expk2}
	&&\text{Var}(\hat k) = \mathbb{E}(\hat k^2) - (\mathbb{E}(\hat k))^2\nonumber\\
	&&= k \alpha_{|\cup(u_1, u_2)|} (1-J_{u_1, u_2})(1 - \alpha_{|\cup(u_1, u_2)|} (1-J_{u_1, u_2})).
	\end{eqnarray}
	From the definition of $\hat J_{u_1, u_2}$, we have
	\begin{equation*}
	\text{Var}(\hat J_{u_1, u_2}) = \text{Var}\left(1 - \frac{\hat k}{k\alpha}\right) = \frac{\text{Var}(\hat k)}{k^2 \alpha^2}.
	\end{equation*}
	Then, we easily obtain a closed-form formals of $\text{Var}(\hat J_{u_1, u_2})$ from equation~(\ref{eq:expk2}).
